# Supplementary material for: Efficient Algorithms for Personalized PageRank
Source: arXiv:1512.04633 source file (2015-12-15)
Supplement: Supplementary file 1 [file appendix1.tex]

\chapter{Appendix 1's Title}
\section{Some section}
Pretty graph!
